# Supplementary material for: Manipulation of the orbital angular momentum of soft x-ray beams by consecutive diffractive optics
Source: arXiv:2511.17768 ancillary file (2025-11-21)
Supplement: Supplementary file 1 [file Supplement_1.pdf]

# Manipulation of the orbital angular momentum of soft x-ray beams by consecutive diffractive optics: supplemental document

NAZIR KHAN[1,*], RAHUL JANGID[2], TARAS STANISLAVCHUK[3], AARON STEIN[4], OLEG CHUBAR[2], ANDI BARBOUR[2], ANDREI SIRENKO[3], VALERY KIRYUKHIN[1], AND CLAUDIO MAZZOLI[2,†]

[1] *Department of Physics and Astronomy, Rutgers University, Piscataway, NJ 08854, USA*
[2] *National Synchrotron Light Source II, Brookhaven National Laboratory, Upton, NY 11973, USA*
[3] *Department of Physics, New Jersey Institute of Technology, Newark, NJ 07102, USA*
[4] *Center for Functional Nanomaterials, Brookhaven National Laboratory, Upton, NY 11973, USA*
[†] *cmazzoli@bnl.gov*
[*] *nazir.khan@rutgers.edu*

## 1. MATERIALS

We produced our fork gratings at the Center for Functional Nanomaterials, Brookhaven National Laboratory, by e-beam lithography on 100 nm thick $Si_3N_4$ membranes using computer generated holograms [1]. The "OAM optics" chip contains a 5×3 matrix of fork gratings [Fig. S1(a)] made

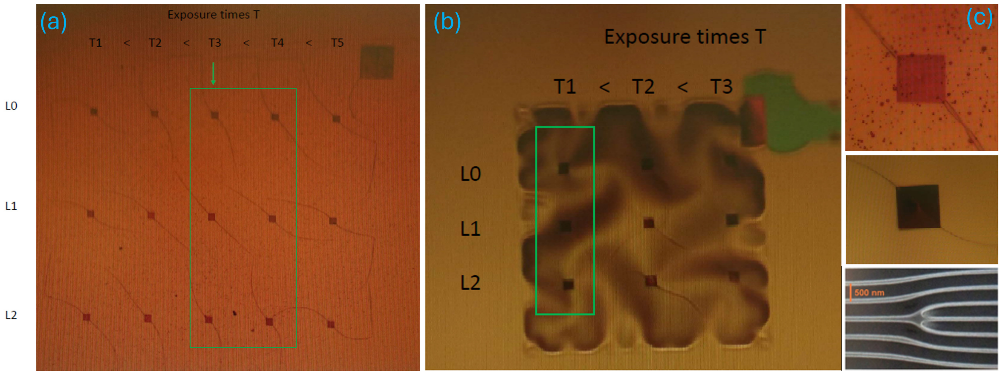


**Fig. S1.** (a) The "OAM optics" chip containing a 5×3 matrix of fork gratings. (b) The "OAM sample" chip containing a 3×3 matrix of fork gratings where the $Si_3N_4$ membrane shows some crumpling. The forks in the first row ($L_0$) have no dislocation defects while the forks in the second ($L_1$) and third ($L_2$) rows have 1 and 2 dislocation defects, respectively. Fork gratings from the green boxes were used for the experiment. (c) Zoomed -in views of a fork grating from the "OAM optics" and "OAM sample" chips (top and middle subpanels, respectively). Bottom subpanel exhibits the SEM image of the 2-fork dislocation grating with a period of 500 nm. The tiny line visible in both top and mid subpanels is a defect on the deposition. The upstream pinhole in our setup mitigates its impact, leaving essentially no trace in our data.

of gold, while the "OAM sample" chip contains a 3×3 matrix of fork gratings [Fig. S1(b)] made of tungsten. Both metal depositions are 300 nm thick and have been Ar milled to excavate the lithographically exposed gratings out of the chemically developed positive photoresist. In both chips, along one direction (rows) of the matrix the OAM charge (L=0, 1, 2) varies, while along

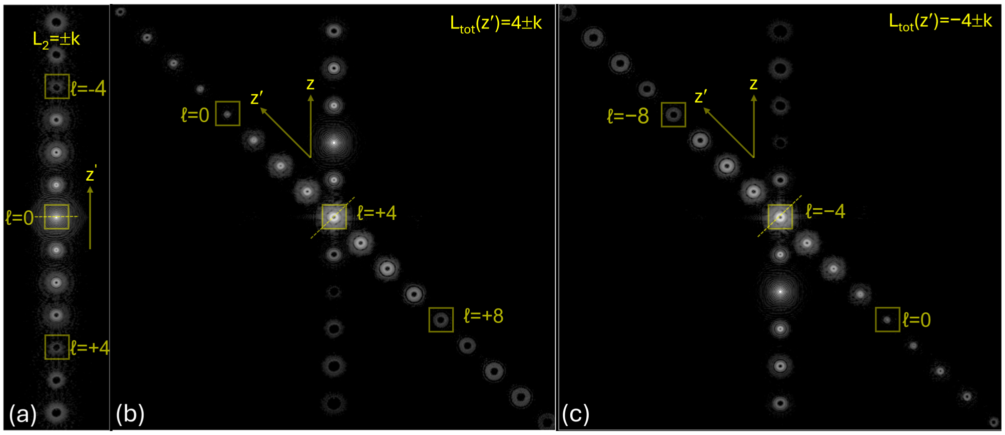


**Fig. S2.** Detector images of the simulated diffraction patterns when a fork grating with one dislocation defect is used as sample (note $z'$) and illuminated by a soft x-ray beam. Panel (a), 45 deg rotated image (for compactness) with no optics upstream, thus using a non-OAM ($\ell$=0) x-ray beam directly from the undulator. Panel (b) and (c), OAM beam of charges $\ell$=+4, and $\ell$=-4, respectively, as generated by a 2-fork grating at the second diffraction order, as an optics (note the position of the gaussian beam along the $z$ axis). The transmitted beam from the sample (1-fork grating) lies on the dashed line (normal to the $z'$-direction). The intensity distribution of different diffraction orders is symmetric w.r.t to the transmitted beam for the non-OAM incident beam (a), whereas it is asymmetric when the incident beam carries an OAM charge ($\ell$=$\pm$4).

the other the e-beam dose (exposure time T) varies, thus allowing to select the best compromise (efficiency versus transmittance) at the selected photon energy. Every grating is contained in a $20\times20\ \mu m^2$ square window, with its symmetry axis rotated by 45 degrees with respect to the sides of the window. This drastically reduces the diffuse scattering generated by the window sides along the grating diffraction direction. All gratings have a period of 500 nm (far from the topological defects). The SEM image of a 2-fork diffraction grating is shown in the bottom panel of Fig. S1(c).

## 2. SIMULATIONS

Start-to-end simulations were done using Synchrotron Radiation Workshop (SRW) electrodynamics and physical optics computer code [2, 3]. It calculates the partially coherent undulator radiation at a given photon energy at beamline entrance, and simulates its propagation, using the methods of Fourier optics (extended to support partial coherence), through the sequence of optical components of the beamline, using accurate models and positions of the reflective and diffractive optics along the beamline, down to the detector. To model the fork gratings, we employed bitmaps that were used for manufacturing of the actual gratings creating the OAM radiation. The detector image of the simulated diffraction pattern spreading along the $z'$-direction for a 1-fork dislocation grating, generating OAM beams with topological charges $L_2$=$\pm$k (in unit of $\hbar$), where $k$ is positive integers when illuminated by a non-OAM x-ray beam, is shown in Fig. S2(a). The intensity distribution is symmetrical on both sides of the central gaussian transmitted beam ($\ell$ =0). Figure S2(b) and S2(c) show the detector images of the simulated diffraction patterns produced by the combination of a 2-fork and a 1-fork dislocation gratings. The diffraction pattern spreading along the $z$- direction is due to the first grating (2-fork) illuminated by non-OAM x-ray beam from the undulator. The OAM beam of topological charge $L_1$=+4$\hbar$ and $L_1$=-4$\hbar$ at the second diffraction orders from the first grating illuminate the second grating (1-fork), resulting in OAM beams spreading along the $z'$ direction with topological charges given by $L_{tot}$=(4$\pm$k)$\hbar$ and $L_{tot}$=(-4$\pm$k)$\hbar$ as shown in Figs. S2(b) and S2(c), respectively. For both the diffraction patterns the intensity distribution is asymmetric on the two sides of the transmitted central OAM beam located at the intersection of $z'$ and $z$, where the non-OAM gaussian beam ($\ell$=0) appears at the 4th diffraction order on the left and right sides of the central beam for $L_{tot}$=(4$\pm$k)$\hbar$ and $L_{tot}$=(-4$\pm$k)$\hbar$, respectively. Also, note the linear increase in the beam size on moving away from the Gaussian beam ($\ell$=0) position.

## REFERENCES


1. S. Li and Z. Wang, Appl. Phys. Lett. **103**, 141110 (2013).
2. O. Chubar, G. Williams, Y. Gao, R. Li, and L. Berman, J. Opt. Soc. Am. A **39**, C240-C252 (2022).
3. SRW GitHub repository
